# Supplementary material for: Stable Attribute Group Editing for Reliable Few-shot Image Generation
Source: arXiv:2302.00179 source file (2023-02-01)
Supplement: Supplementary file 1 [file Appendix.tex]

\clearpage

\appendix
\appendices

\section{Demonstration of the Assumption of Gaussian Distribution }
\label{gaussian}
\begin{figure}[t]
\centering
     \includegraphics[width=\linewidth]{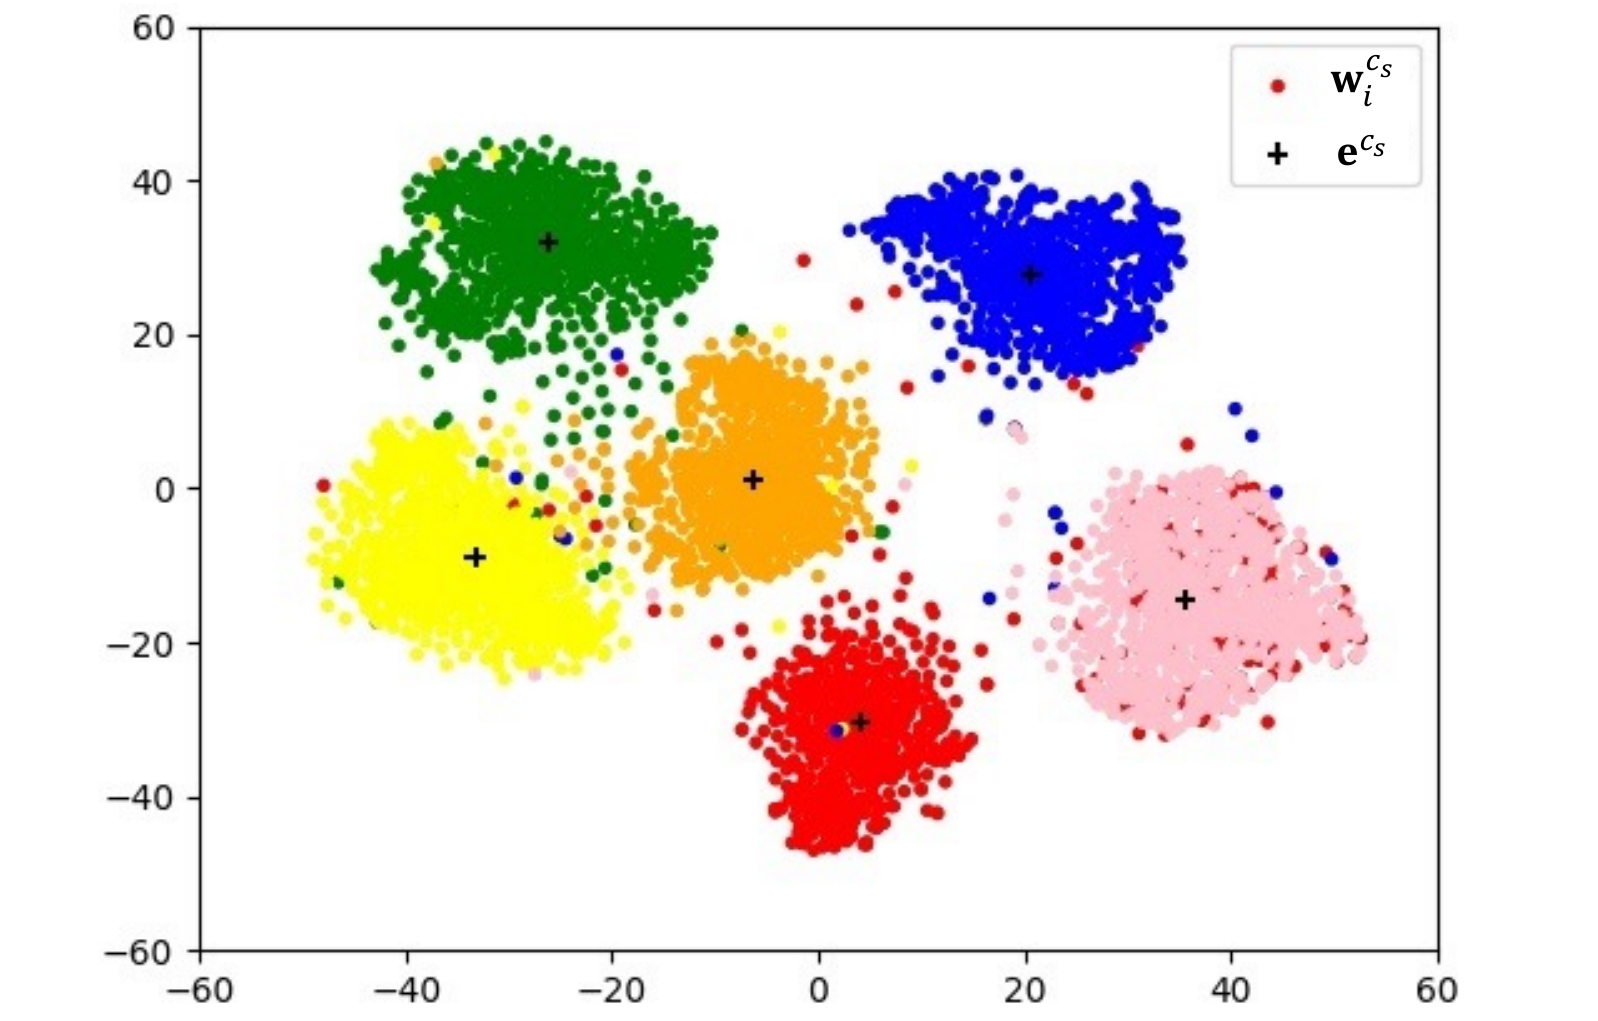}
     \vspace{-2em}
    \caption{Visualization of $\mathcal{W^+}$ space after TSNE.}
    \label{gaussian_distribution}
\end{figure}

We make an assumption that the distribution of the samples in $\mathcal{W^+}$ space obeys Gaussian distribution in Eq. 15.
This assumption is from StyleGAN that different images can be generated from a center image with linearly interpolation along different directions in the embedding space.
In Fig.~\ref{gaussian_distribution}, we further illustrate the latent embeddings of samples from 6 different categories after TSNE. The distribution of different categories indeed roughly follows the Gaussian distribution.

\section{Comparison with Unsupervised Image Manipulation Methods }
\label{sefa}
\begin{figure*}[t]
\centering
     \includegraphics[width=0.65\linewidth]{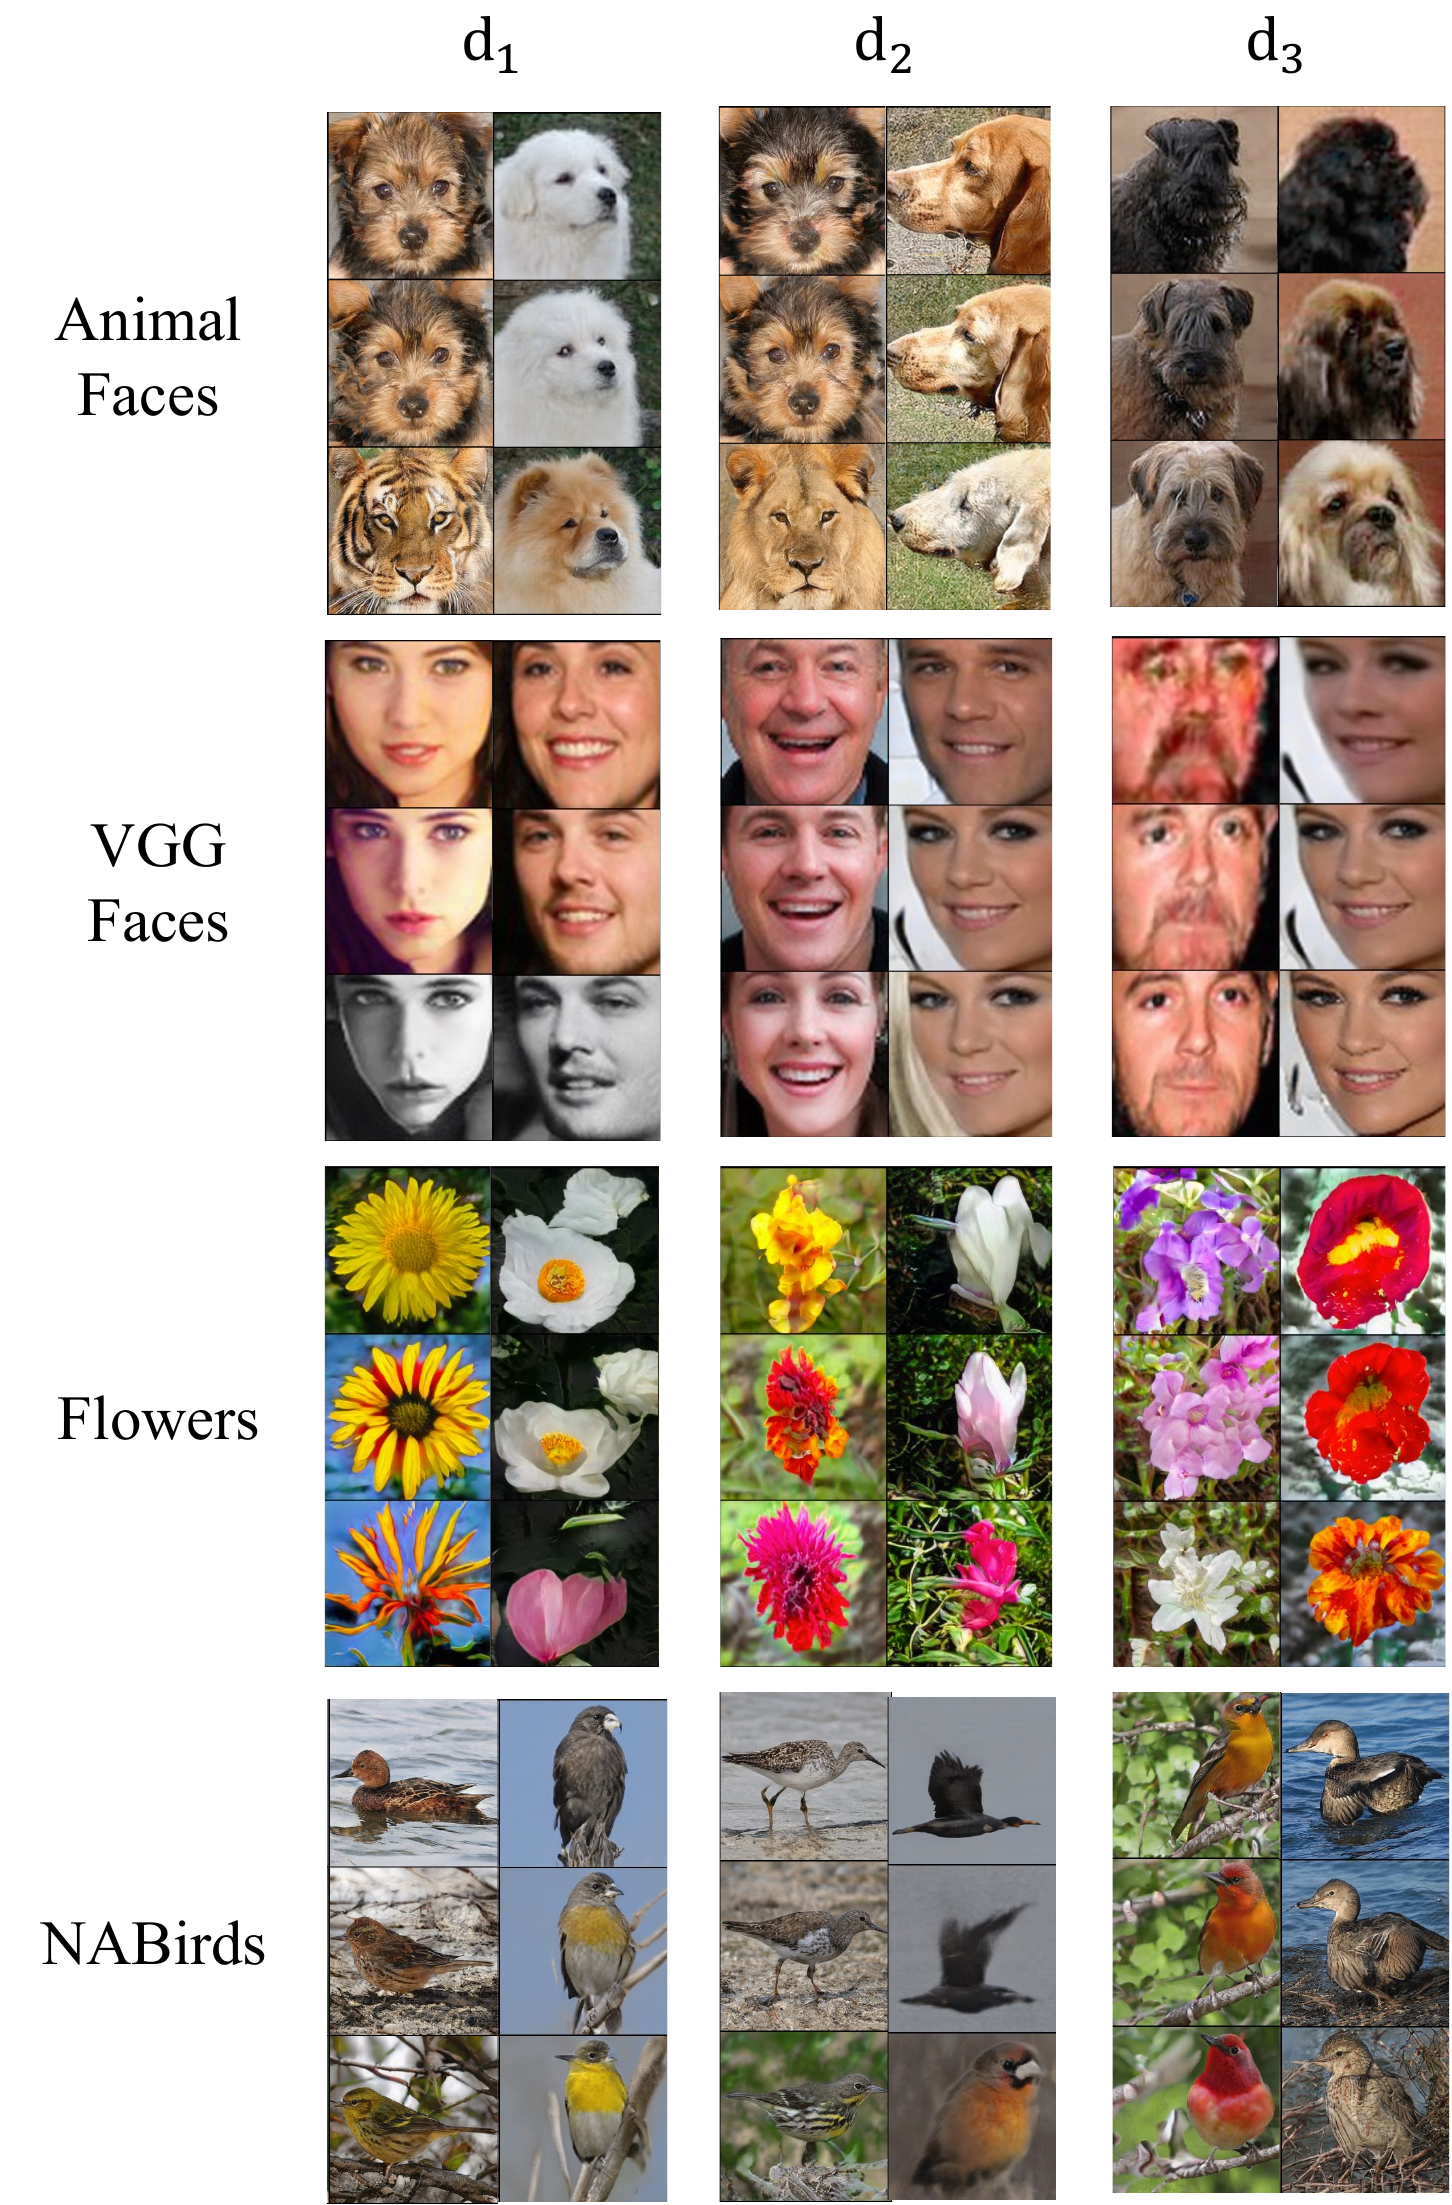}
    \caption{Visualizations of interpretable directions discovered by SeFa. The middle and bottom right images are edited from the top one.
    Moving the latent vectors along the discovered directions apparently changes the categories of the images.}
    \label{image_editing_comparison}
\end{figure*}

The core of the editing-based few-shot image generation is to identify the category-relevant and category-irrelevant attributes in the latent space without explicit supervision.
Similar to SAGE, unsupervised image manipulation methods~\cite{sefa,RW11-Hessian,jacobian} also utilize the semantic factorization of a pre-trained GAN. 
However, they only focus on single-category image generation and do not care about the categorical information.
In order to verify if they can distinguish the category-irrelevant directions for few-shot image generation, we evaluate the recent proposed method SeFa~\cite{sefa} on three multi-class image generation datasets.
SeFa performs a closed-form factorization on the latent semantics according to the weights of the generator, which is one of the best unsupervised attribute factorization and manipulation methods.

Fig.~\ref{image_editing_comparison} shows the first three directions discovered by SeFa. In complicated datasets Animal Faces~\cite{animalfaces}, Flowers~\cite{flowers} and NABirds~\cite{nabirds}, the category-irrelevant attributes and category-relevant attributes are all entangled. 
The semantics in the interpreted directions by SeFa are hard to distinguish.
Editing along a single direction changes multiple attributes and results in an image of a completely different category (\eg, from \texttt{dog} to \texttt{tiger}, the shape of the petals, from \texttt{eagle} to \texttt{finch}, {\it etc.}). In VGGFaces~\cite{vggfaces}, despite achieving better disentanglement, the top important semantics discovered by SeFa are almost category-relevant including the sex and the shape of the face. In contrast, SAGE can factorize the category-irrelevant attributes from the category-relevant attributes, which is the most important for few-shot image generation.

\subsection{Controllable Editing}%根据篇幅决定是否保留
Since editing-based methods fully exploit the interpretability of GAN's latent space, the directions in the dictionary $\bf{A}$ are semantically meaningful.
Therefore, an additional advantage for AGE and SAGE is controllable image editing with respect to the category-irrelevant attributes. 
In this section, we will experimentally demonstrate the transferability and interpretability of the learned dictionary $\bf{A}$.

\subsubsection{Transferability}
Since $\bf{A}$ is learned across all categories in the training set, the directions in $\bf{A}$ is transferable across different %seen and unseen 
categories. We edit the images from 4 categories with the same editing direction, the output images are shown in Fig.~\ref{trans}. 
\texttt{Trans1} is to open the mouth and \texttt{Trans2} is to turn the head to right. It demonstrates that the dictionary $\bf{A}$ is global and the same $\mathbf{n}$ controls similar attributes for images of different categories. 

\begin{figure}[t]
	\centering
	\includegraphics[width=0.9\linewidth]{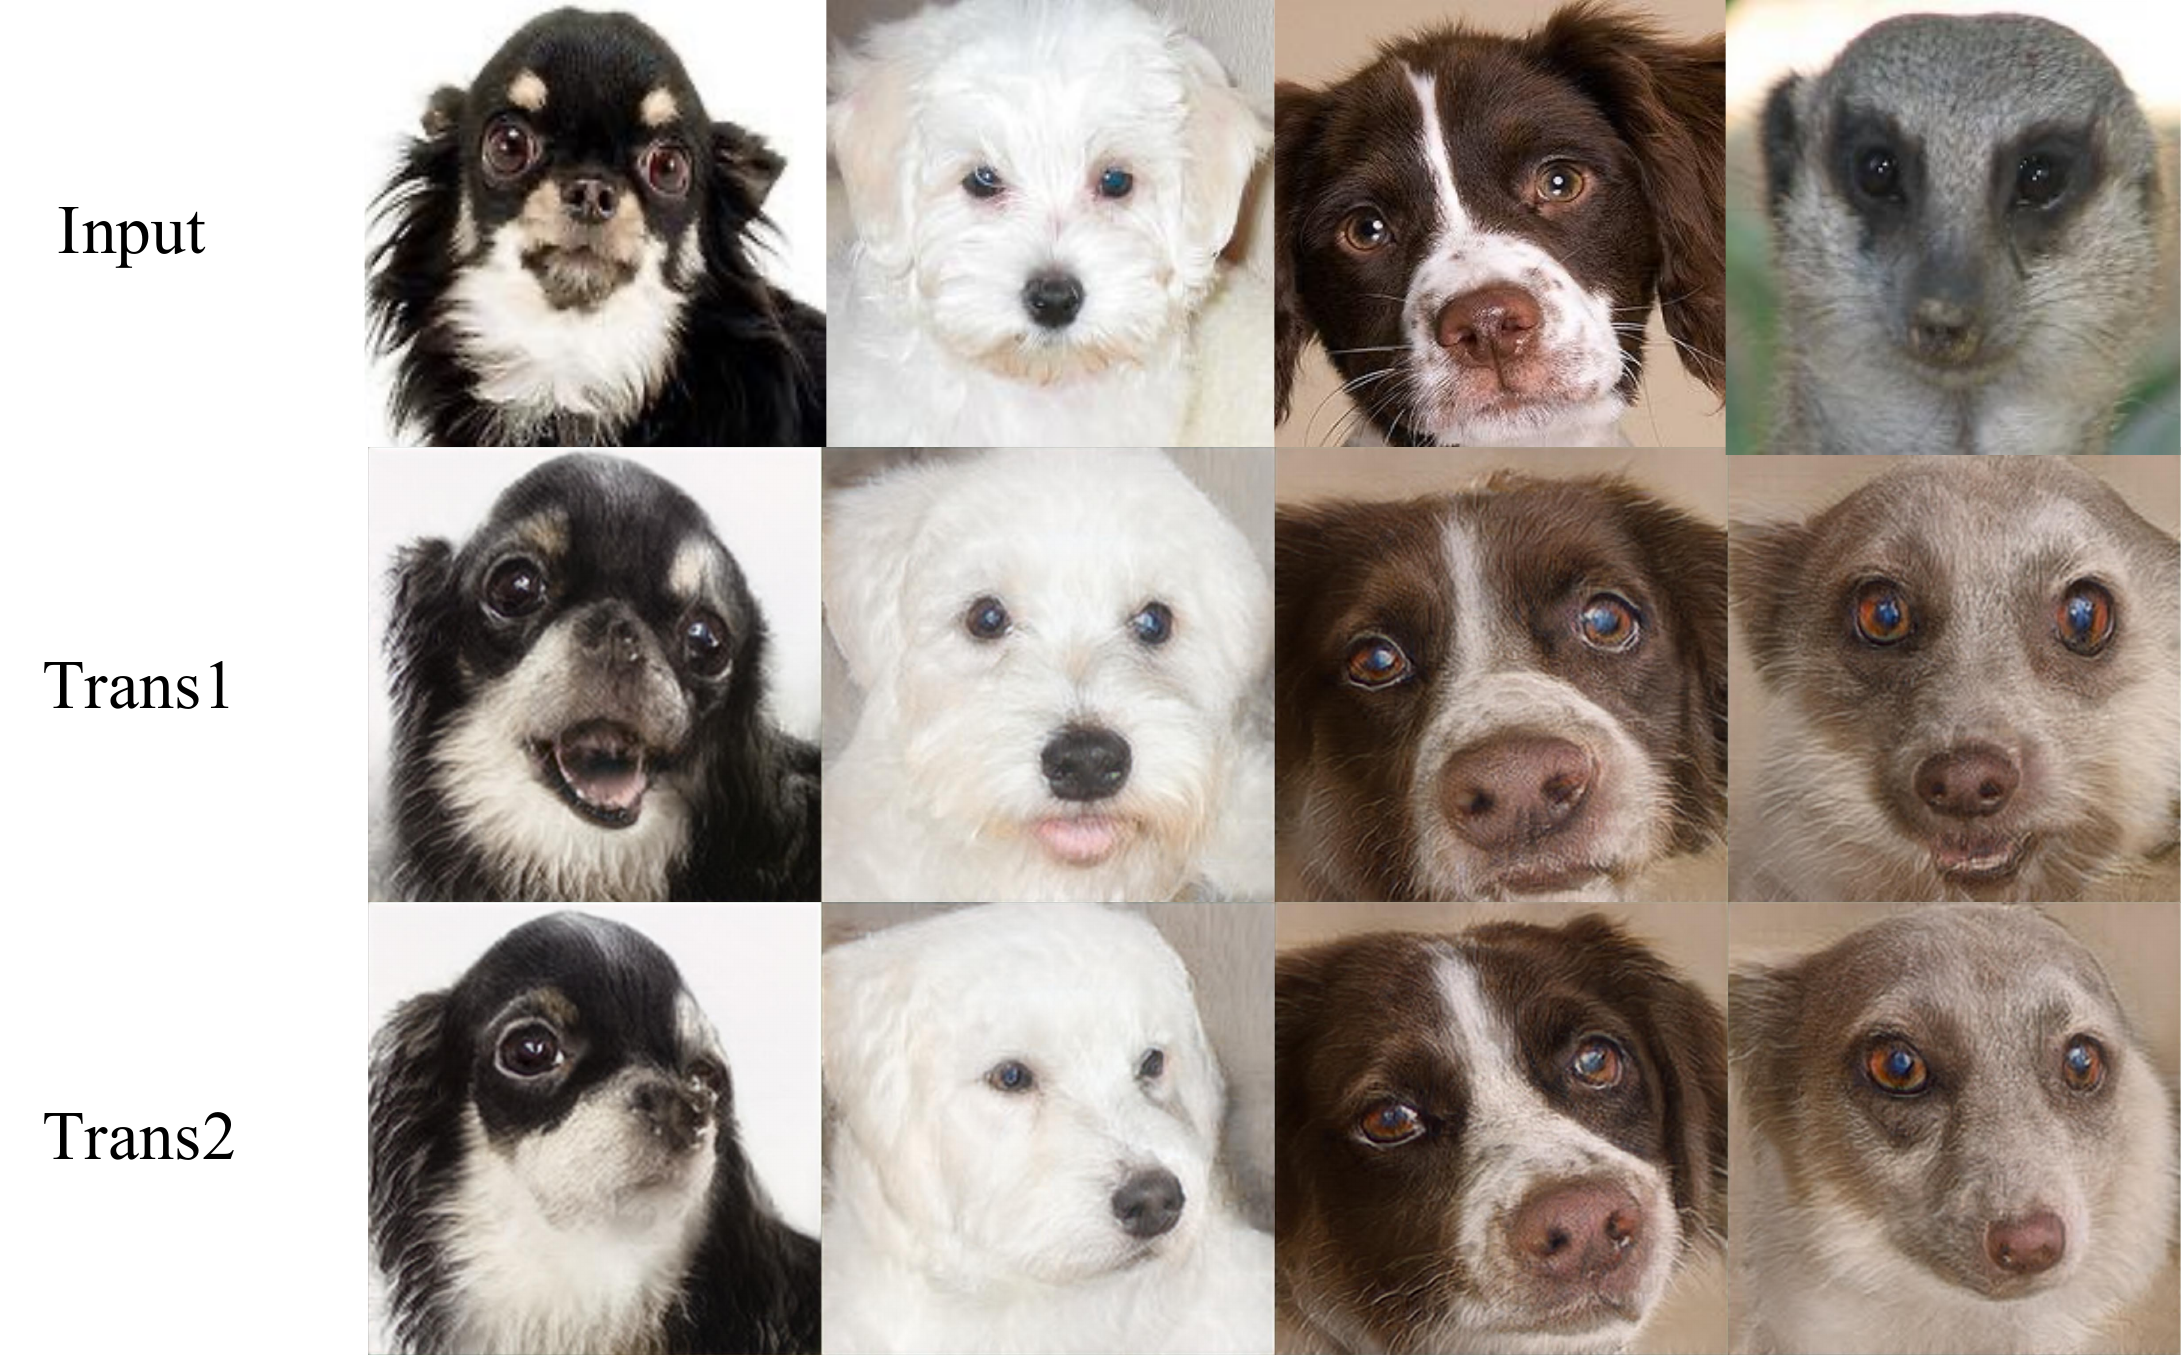}
	\caption{Manipulate images from different categories with the same sparse representation $\bf{n}$.}
	\vspace{-0.8em}
	\label{trans}
\end{figure}

\subsubsection{Interpretability} 
SAGE performs semantic disentanglement in a completely self-supervised manner, the learned directions in $\bf{A}$ are interpretable due to the sparse constraint and the meaningful latent space of StyleGAN2.

First, different groups of layers control different category-irrelevant attributes. In particular, we interpret a target model at the bottom layers, middle layers, and top layers, respectively. Fig.~\ref{hierarchichal_editing} shows the versatile semantic directions found in Animal Faces. 
It demonstrates that most directions in $\bf{A}$ is category-irrelevant.
Concretely, the bottom layers mainly control the structure of objects, such as the position, zoom in/out, and the shape of the face. The middle layers mainly control the surface features like color and the expressions. The top layers decide the background and the overall hue of the image. SAGE can achieve controllable category-irrelevant editing by sampling in corresponding groups.

To find the disentangled attribute editing directions in different layers/groups, we further conduct singular value decomposition on dictionary ${\bf A}$:
\begin{equation}
    {\bf A} = {\bf U}_{ A} {\bf \Sigma} {\bf V}^*.
\end{equation}
The matrix ${\bf U}_A$ contains the commonly shared directions of each layer of dictionary $\bf{A}$. Fig.~\ref{svd} is an illustration of image editing by moving along the most salient directions of each layer. Although the disentanglement is rough, moving along a single direction in ${\bf U}_A$ can enable the continuous editing on one specific category-irrelevant attribute.

\begin{figure}[t]
	\centering
	\includegraphics[width=\linewidth]{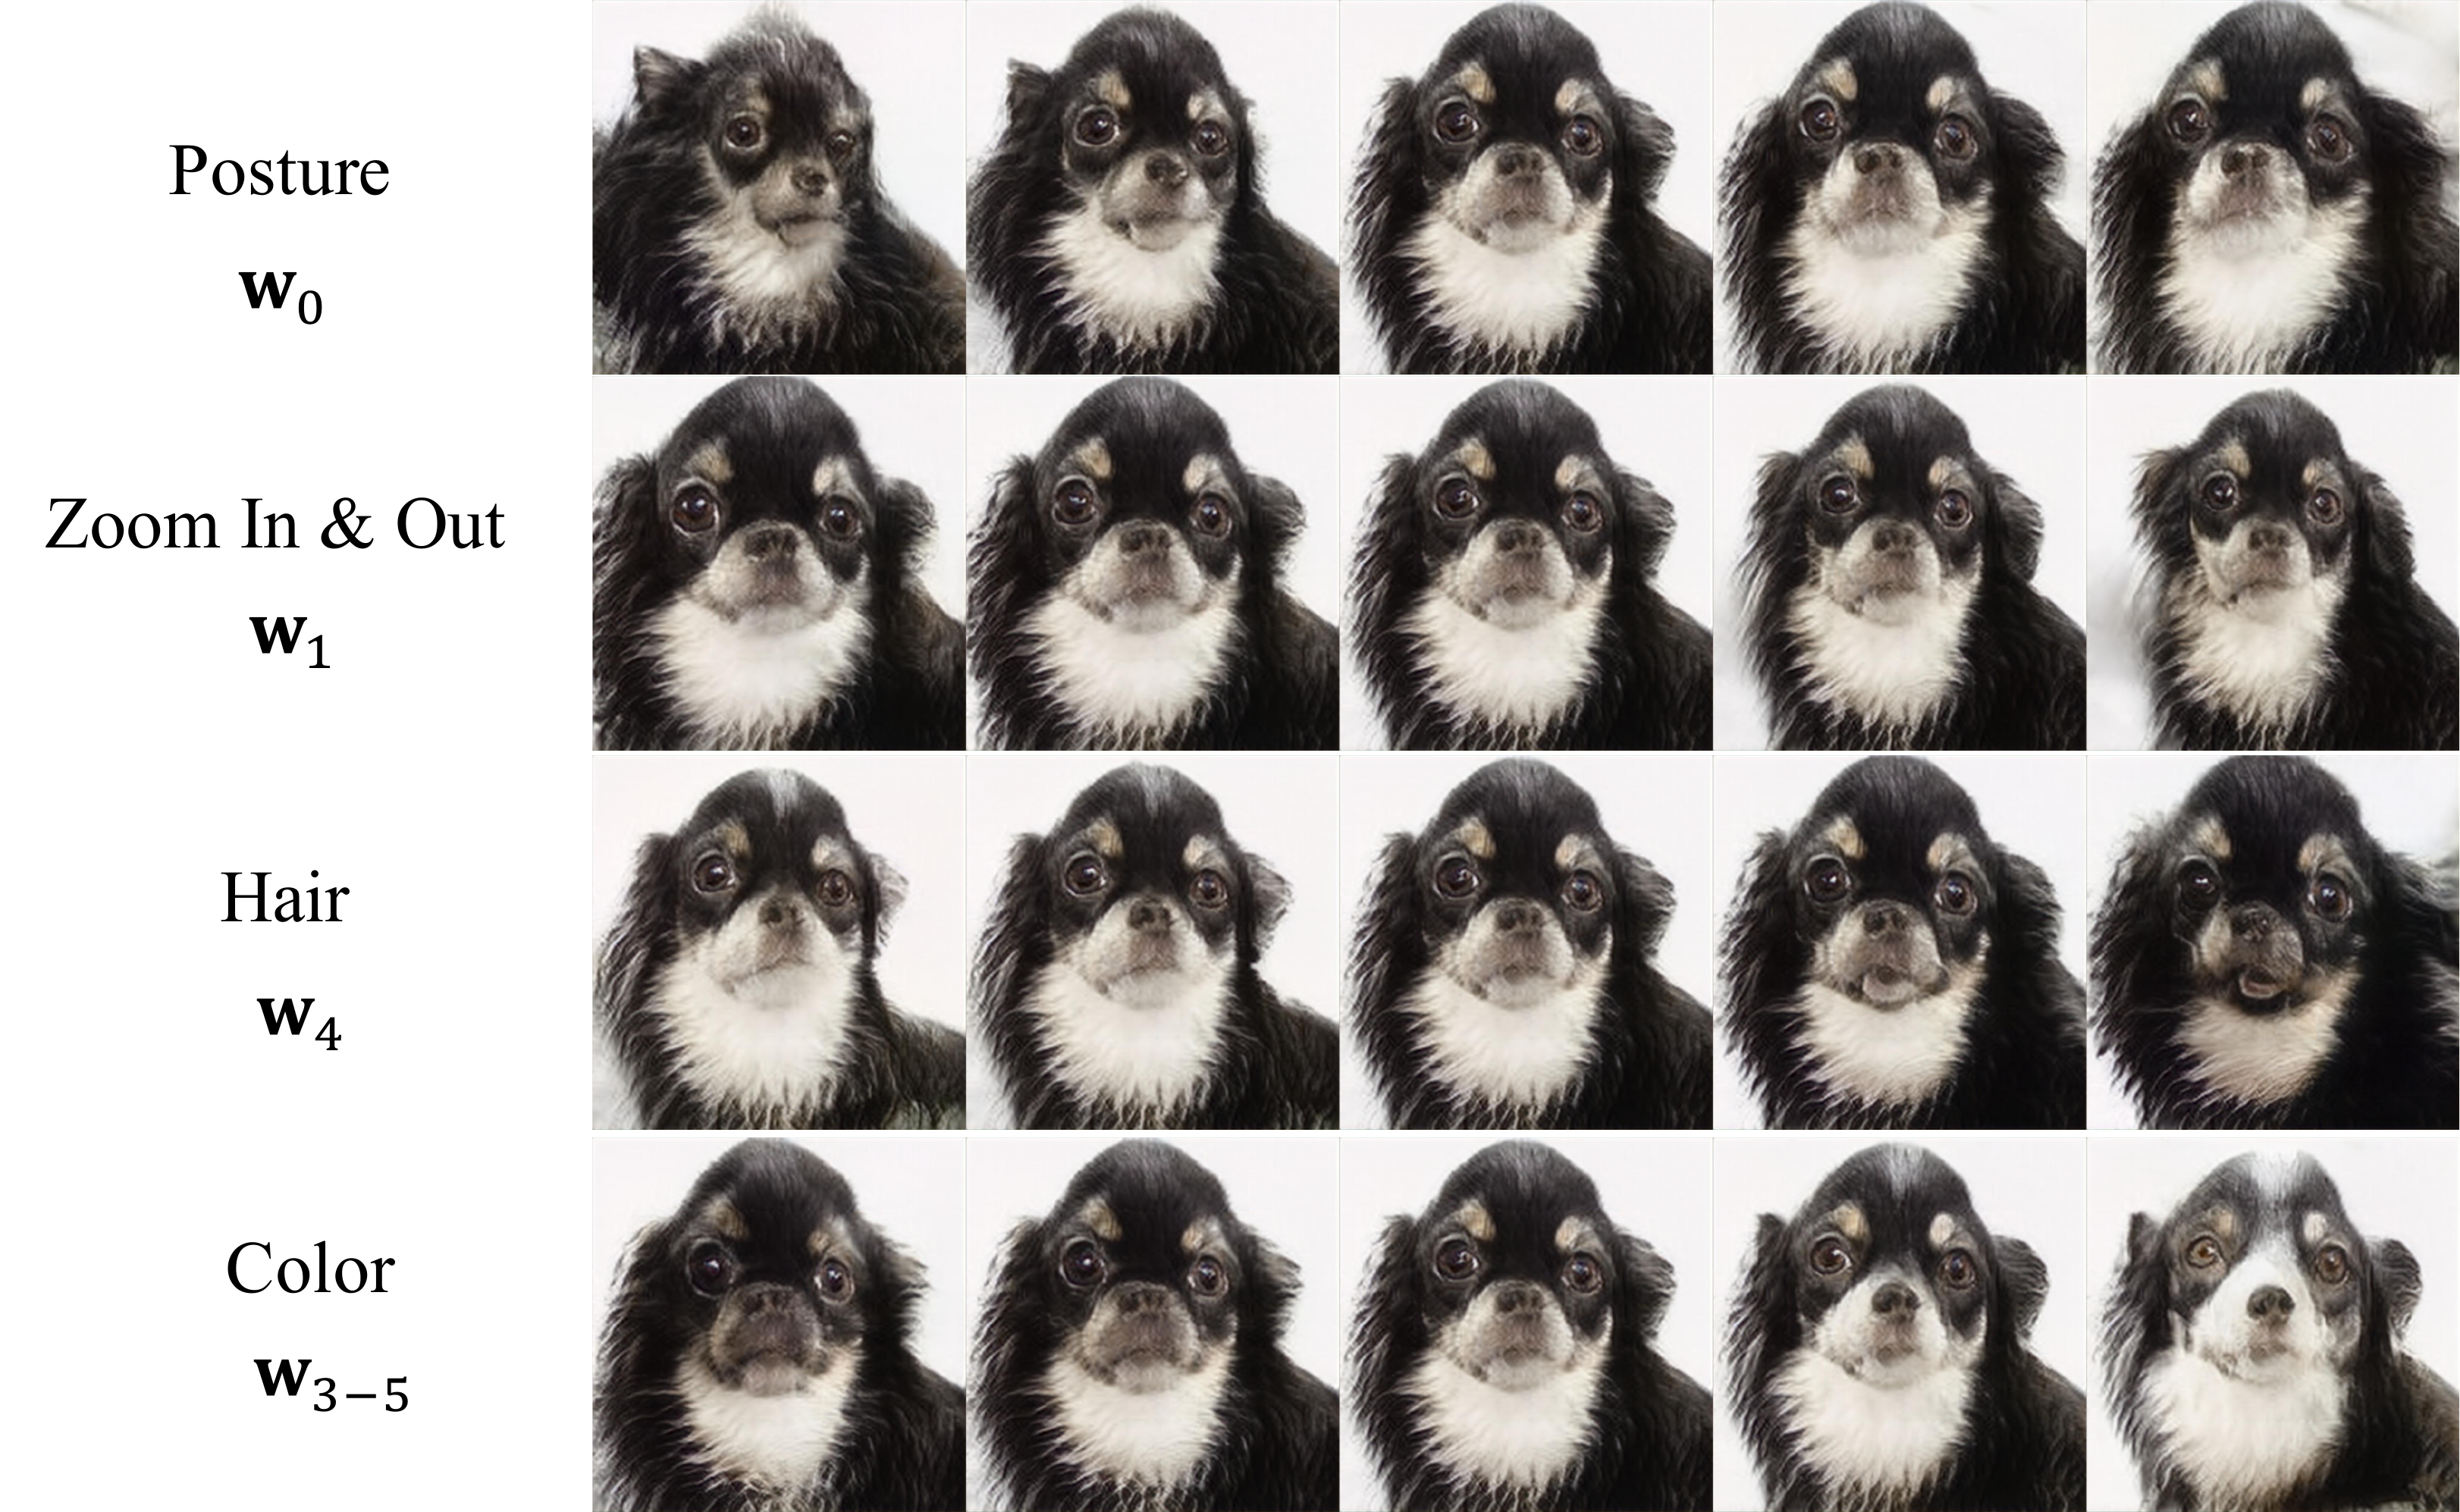}
	\caption{Illustration of image manipulation along disentangled attribute editing directions in different layers in $\bf{U}$.}

	\label{svd}
\end{figure}

\begin{figure*}[t]
	\centering
	\includegraphics[width=0.9\linewidth]{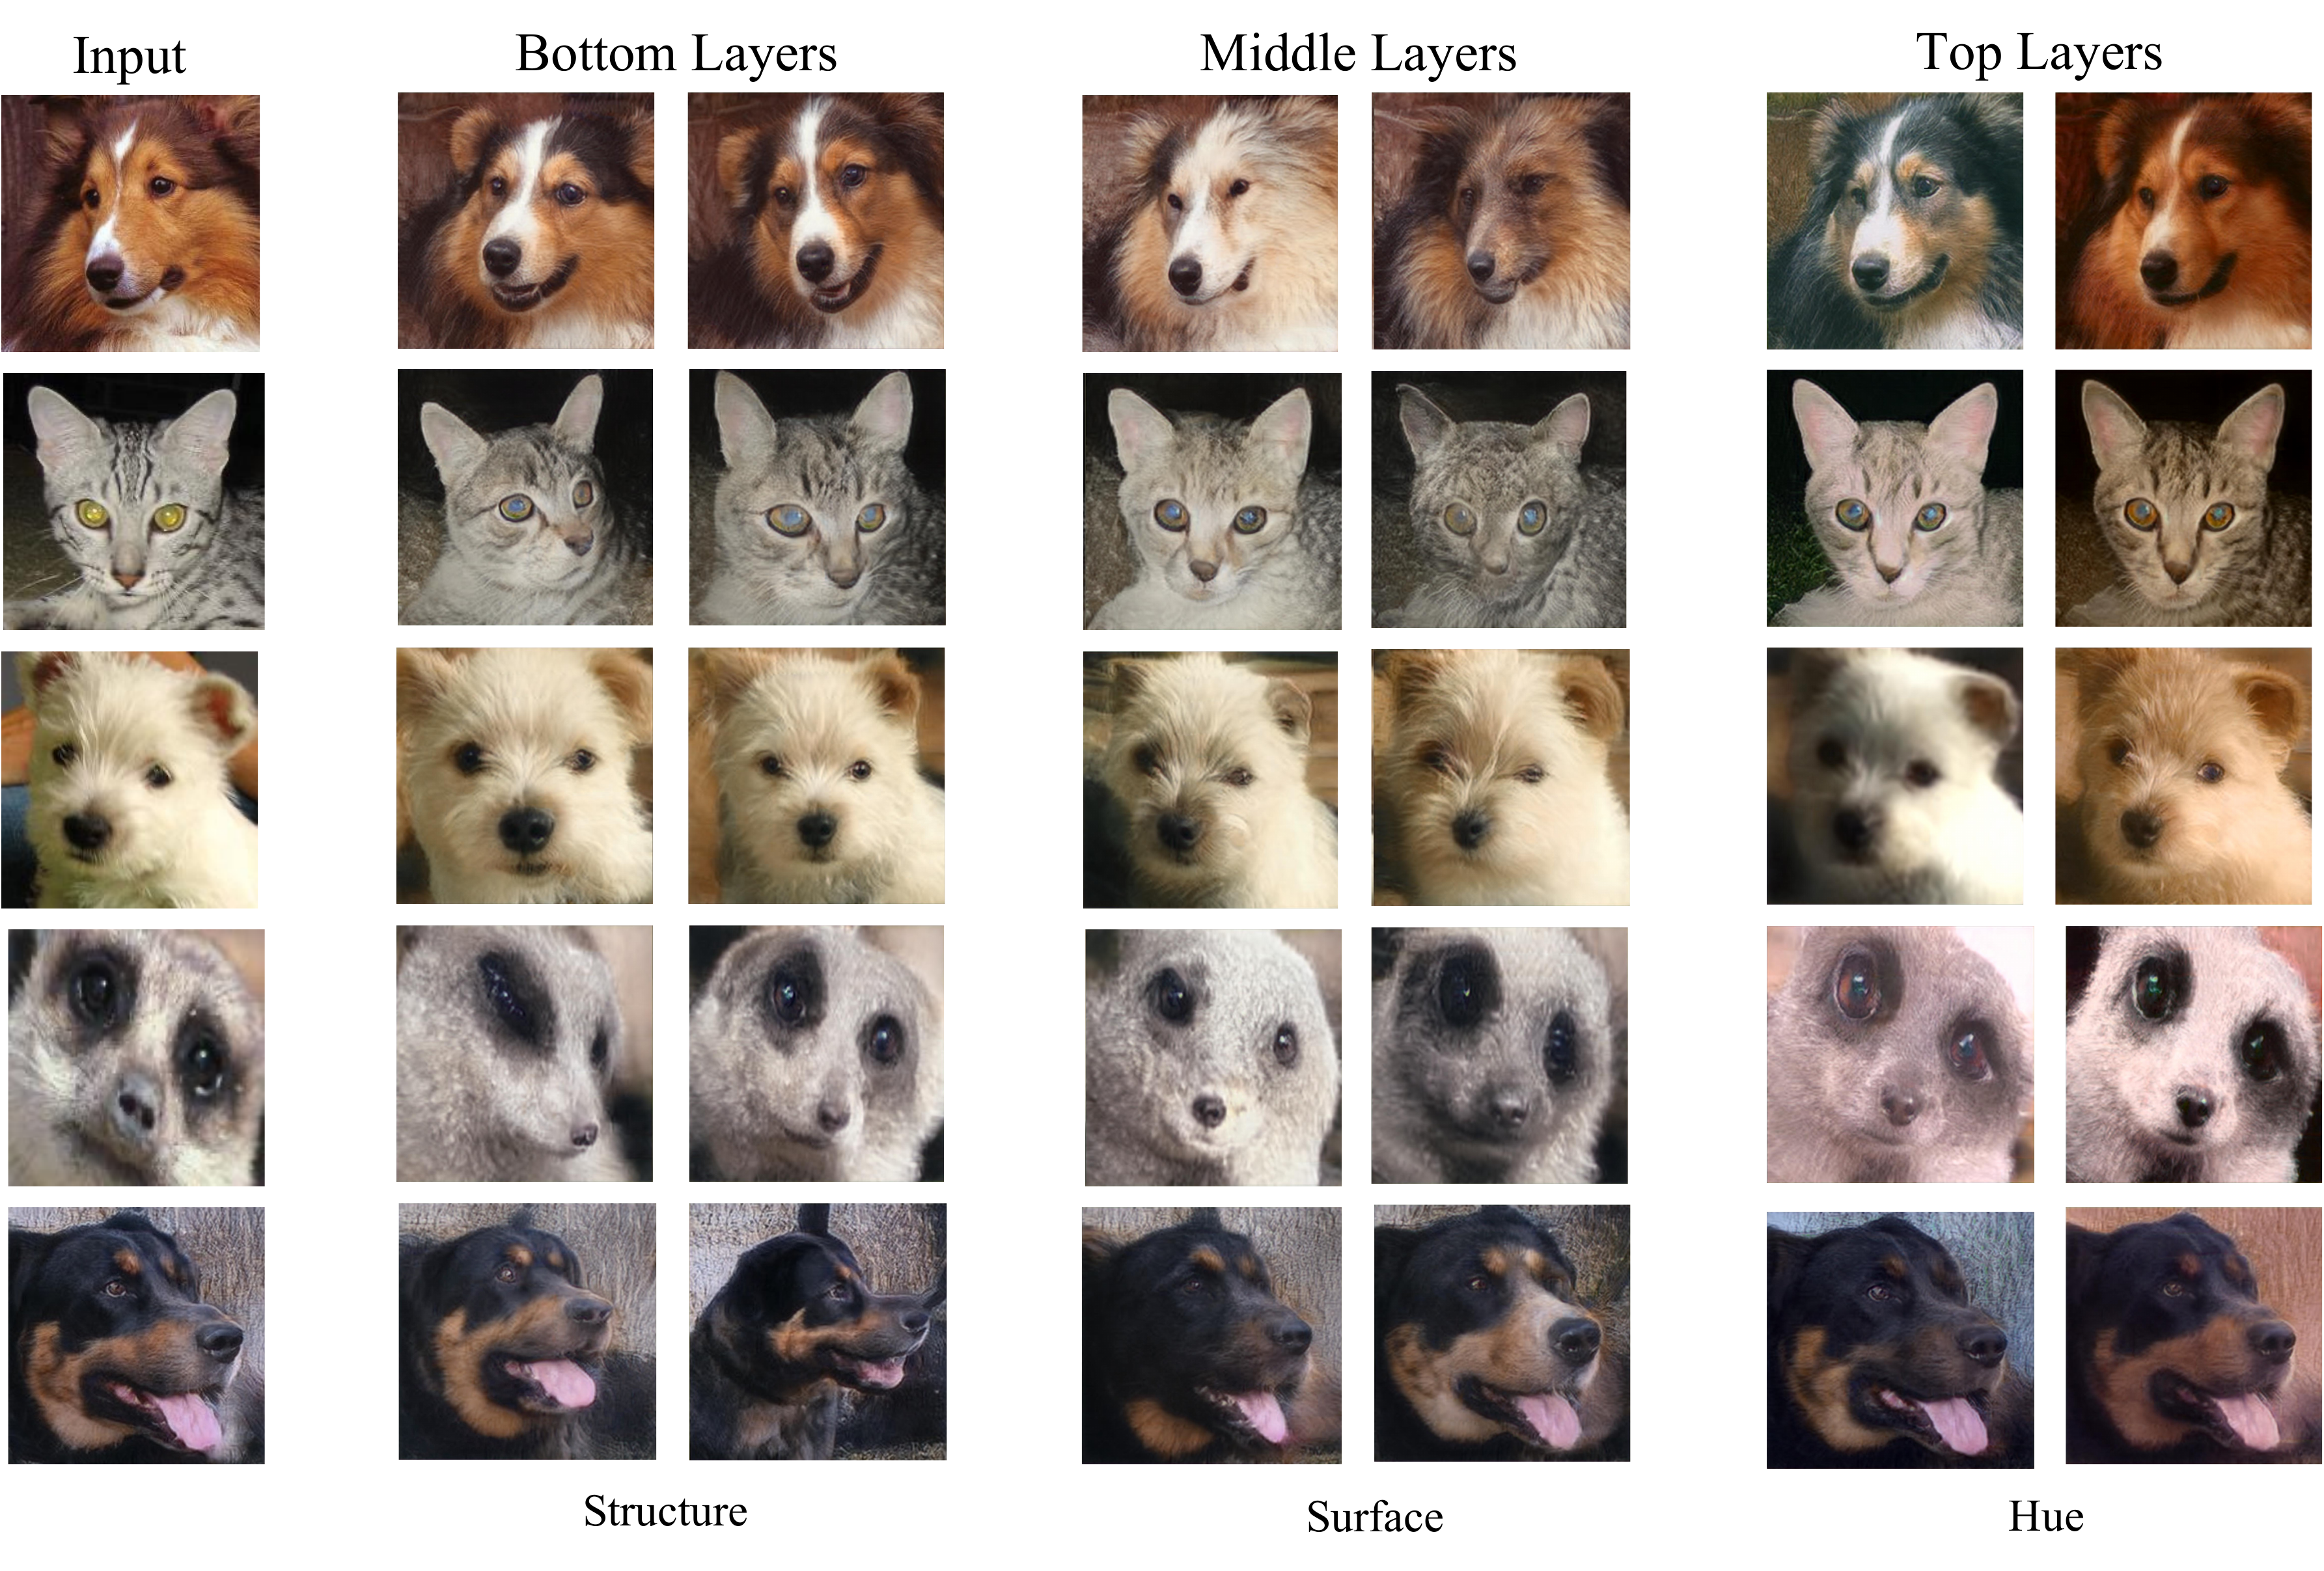}
	\caption{Hierarchical interpretable manipulations discovered in $\bf{A}$.}

	\label{hierarchichal_editing}
\end{figure*}

\begin{figure*}[ht]
    \centering
    \includegraphics[width=0.9\linewidth]{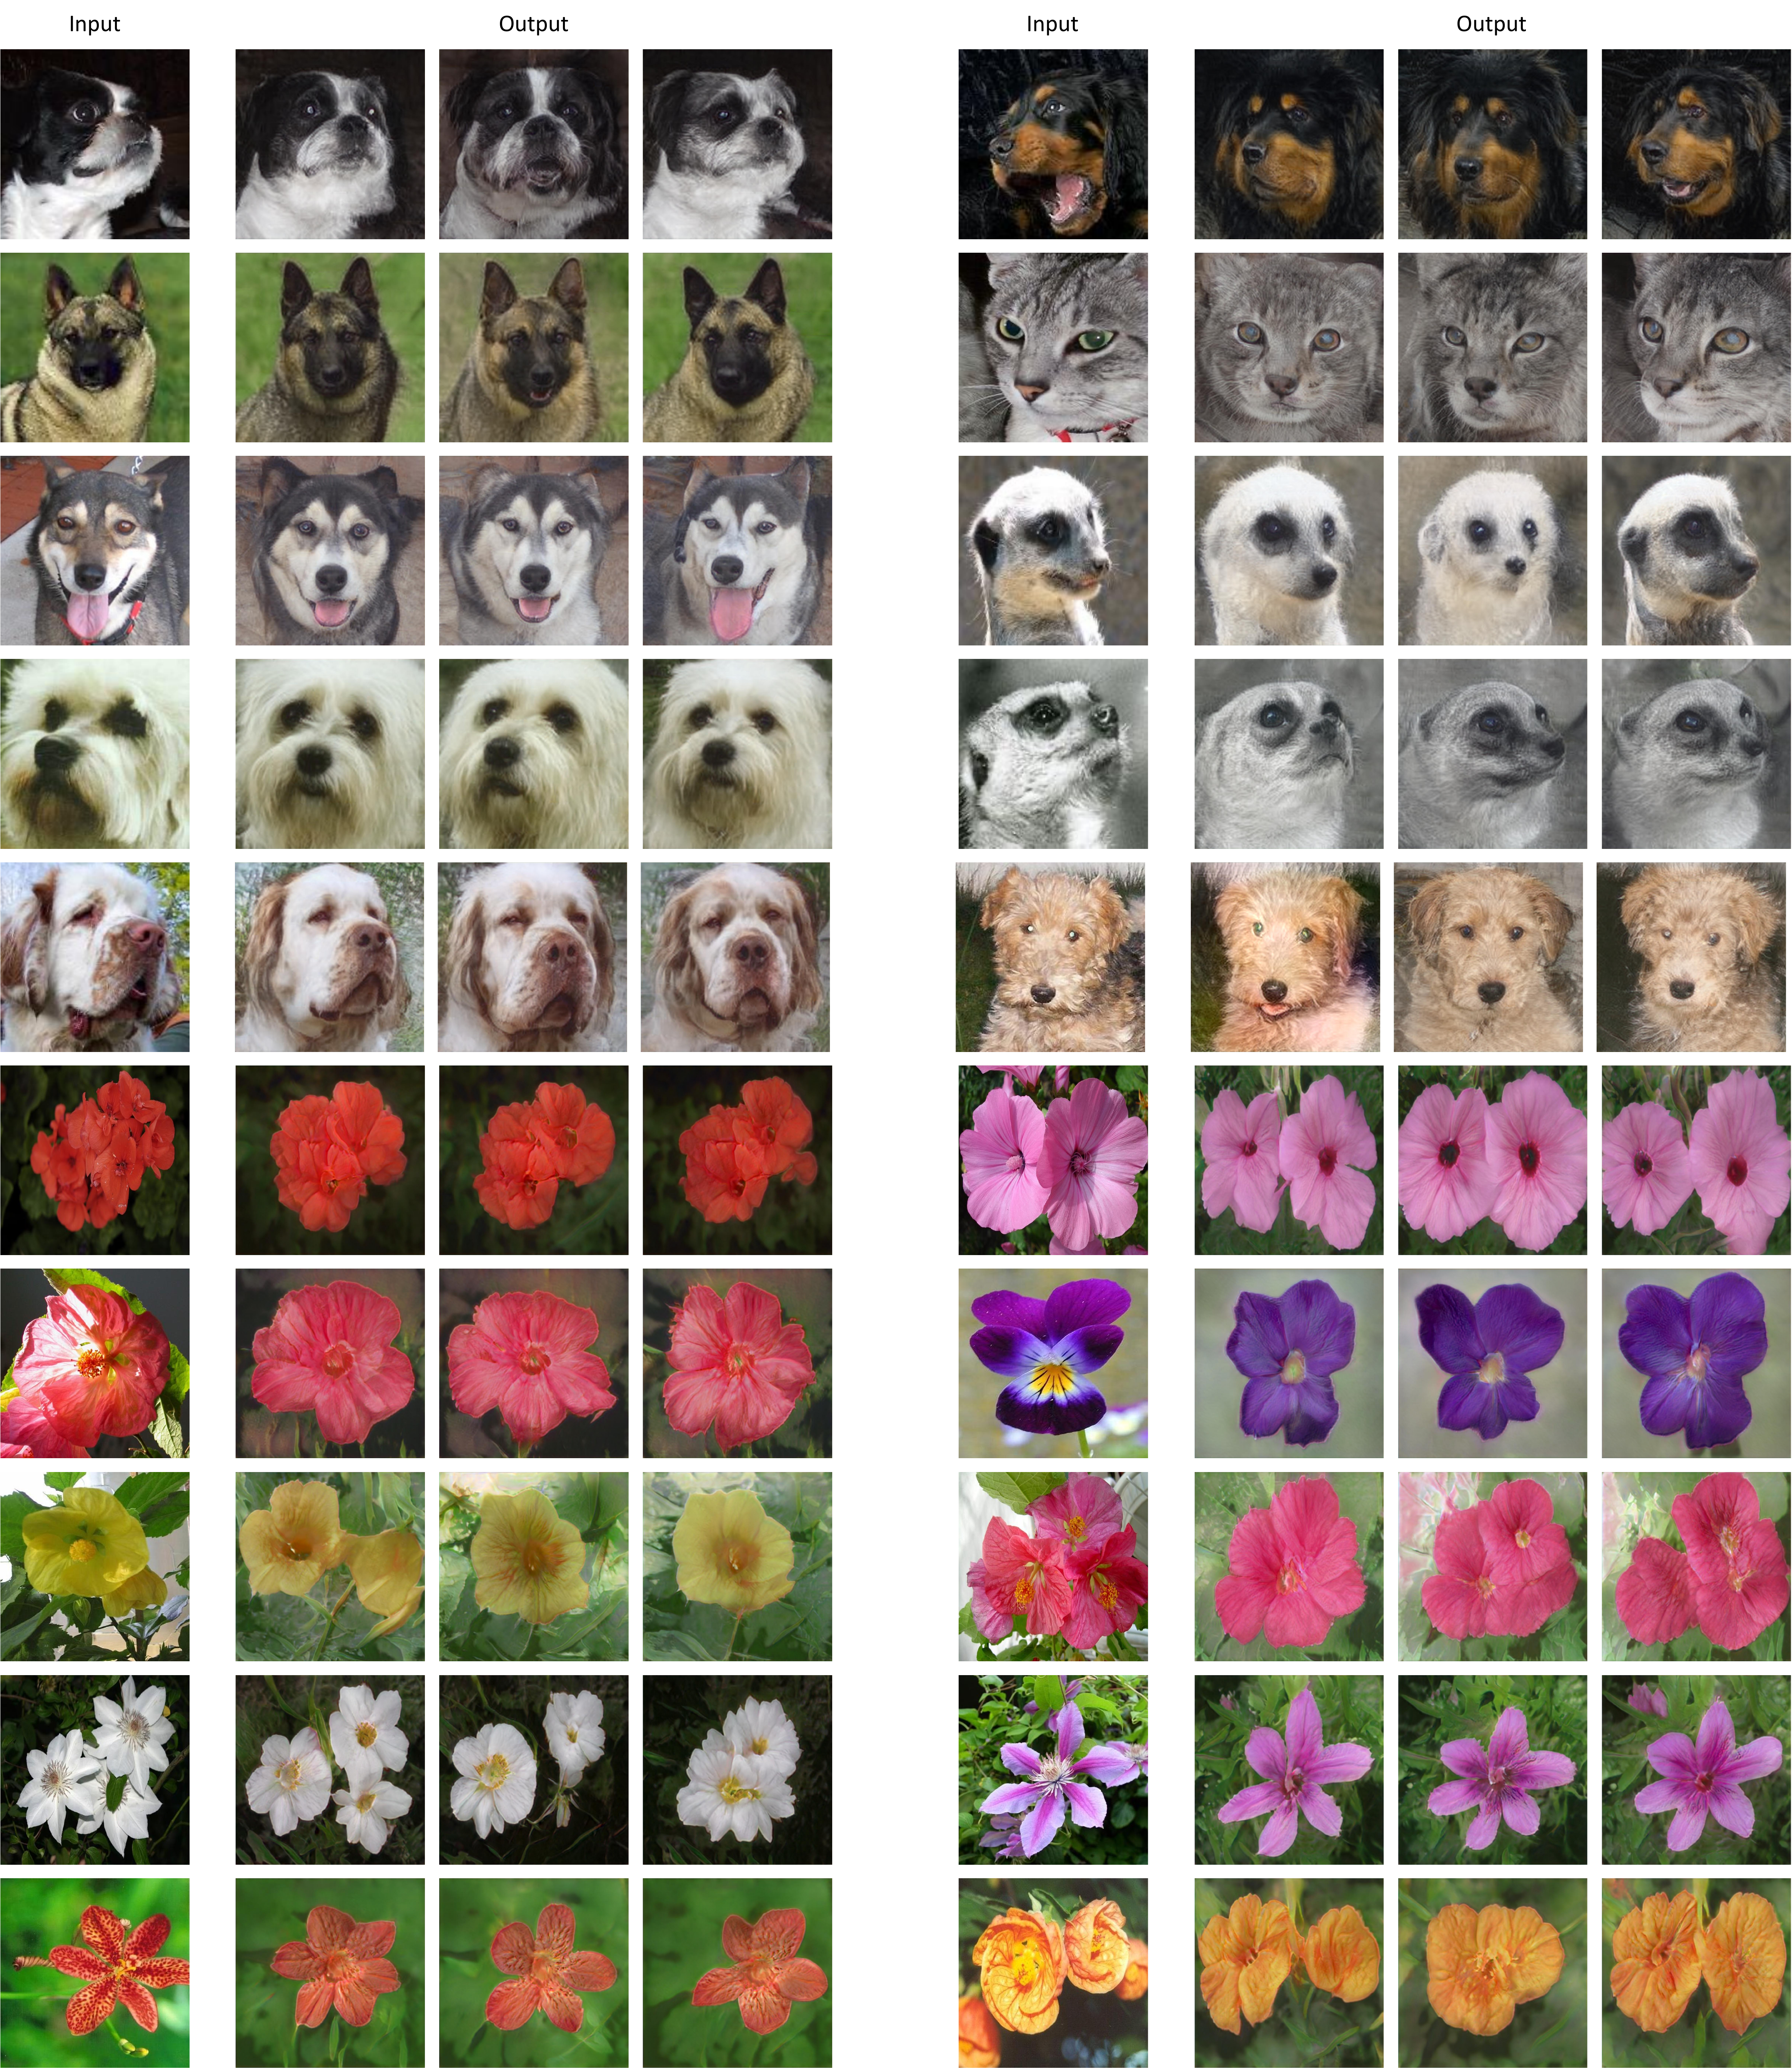}

    \caption{Images generated by SAGE under 1-shot setting on Animal Faces and Flowers.}
    \label{1-shot_samples0}
\end{figure*}

\begin{figure*}[ht]
    \centering
    \includegraphics[width=0.9\linewidth]{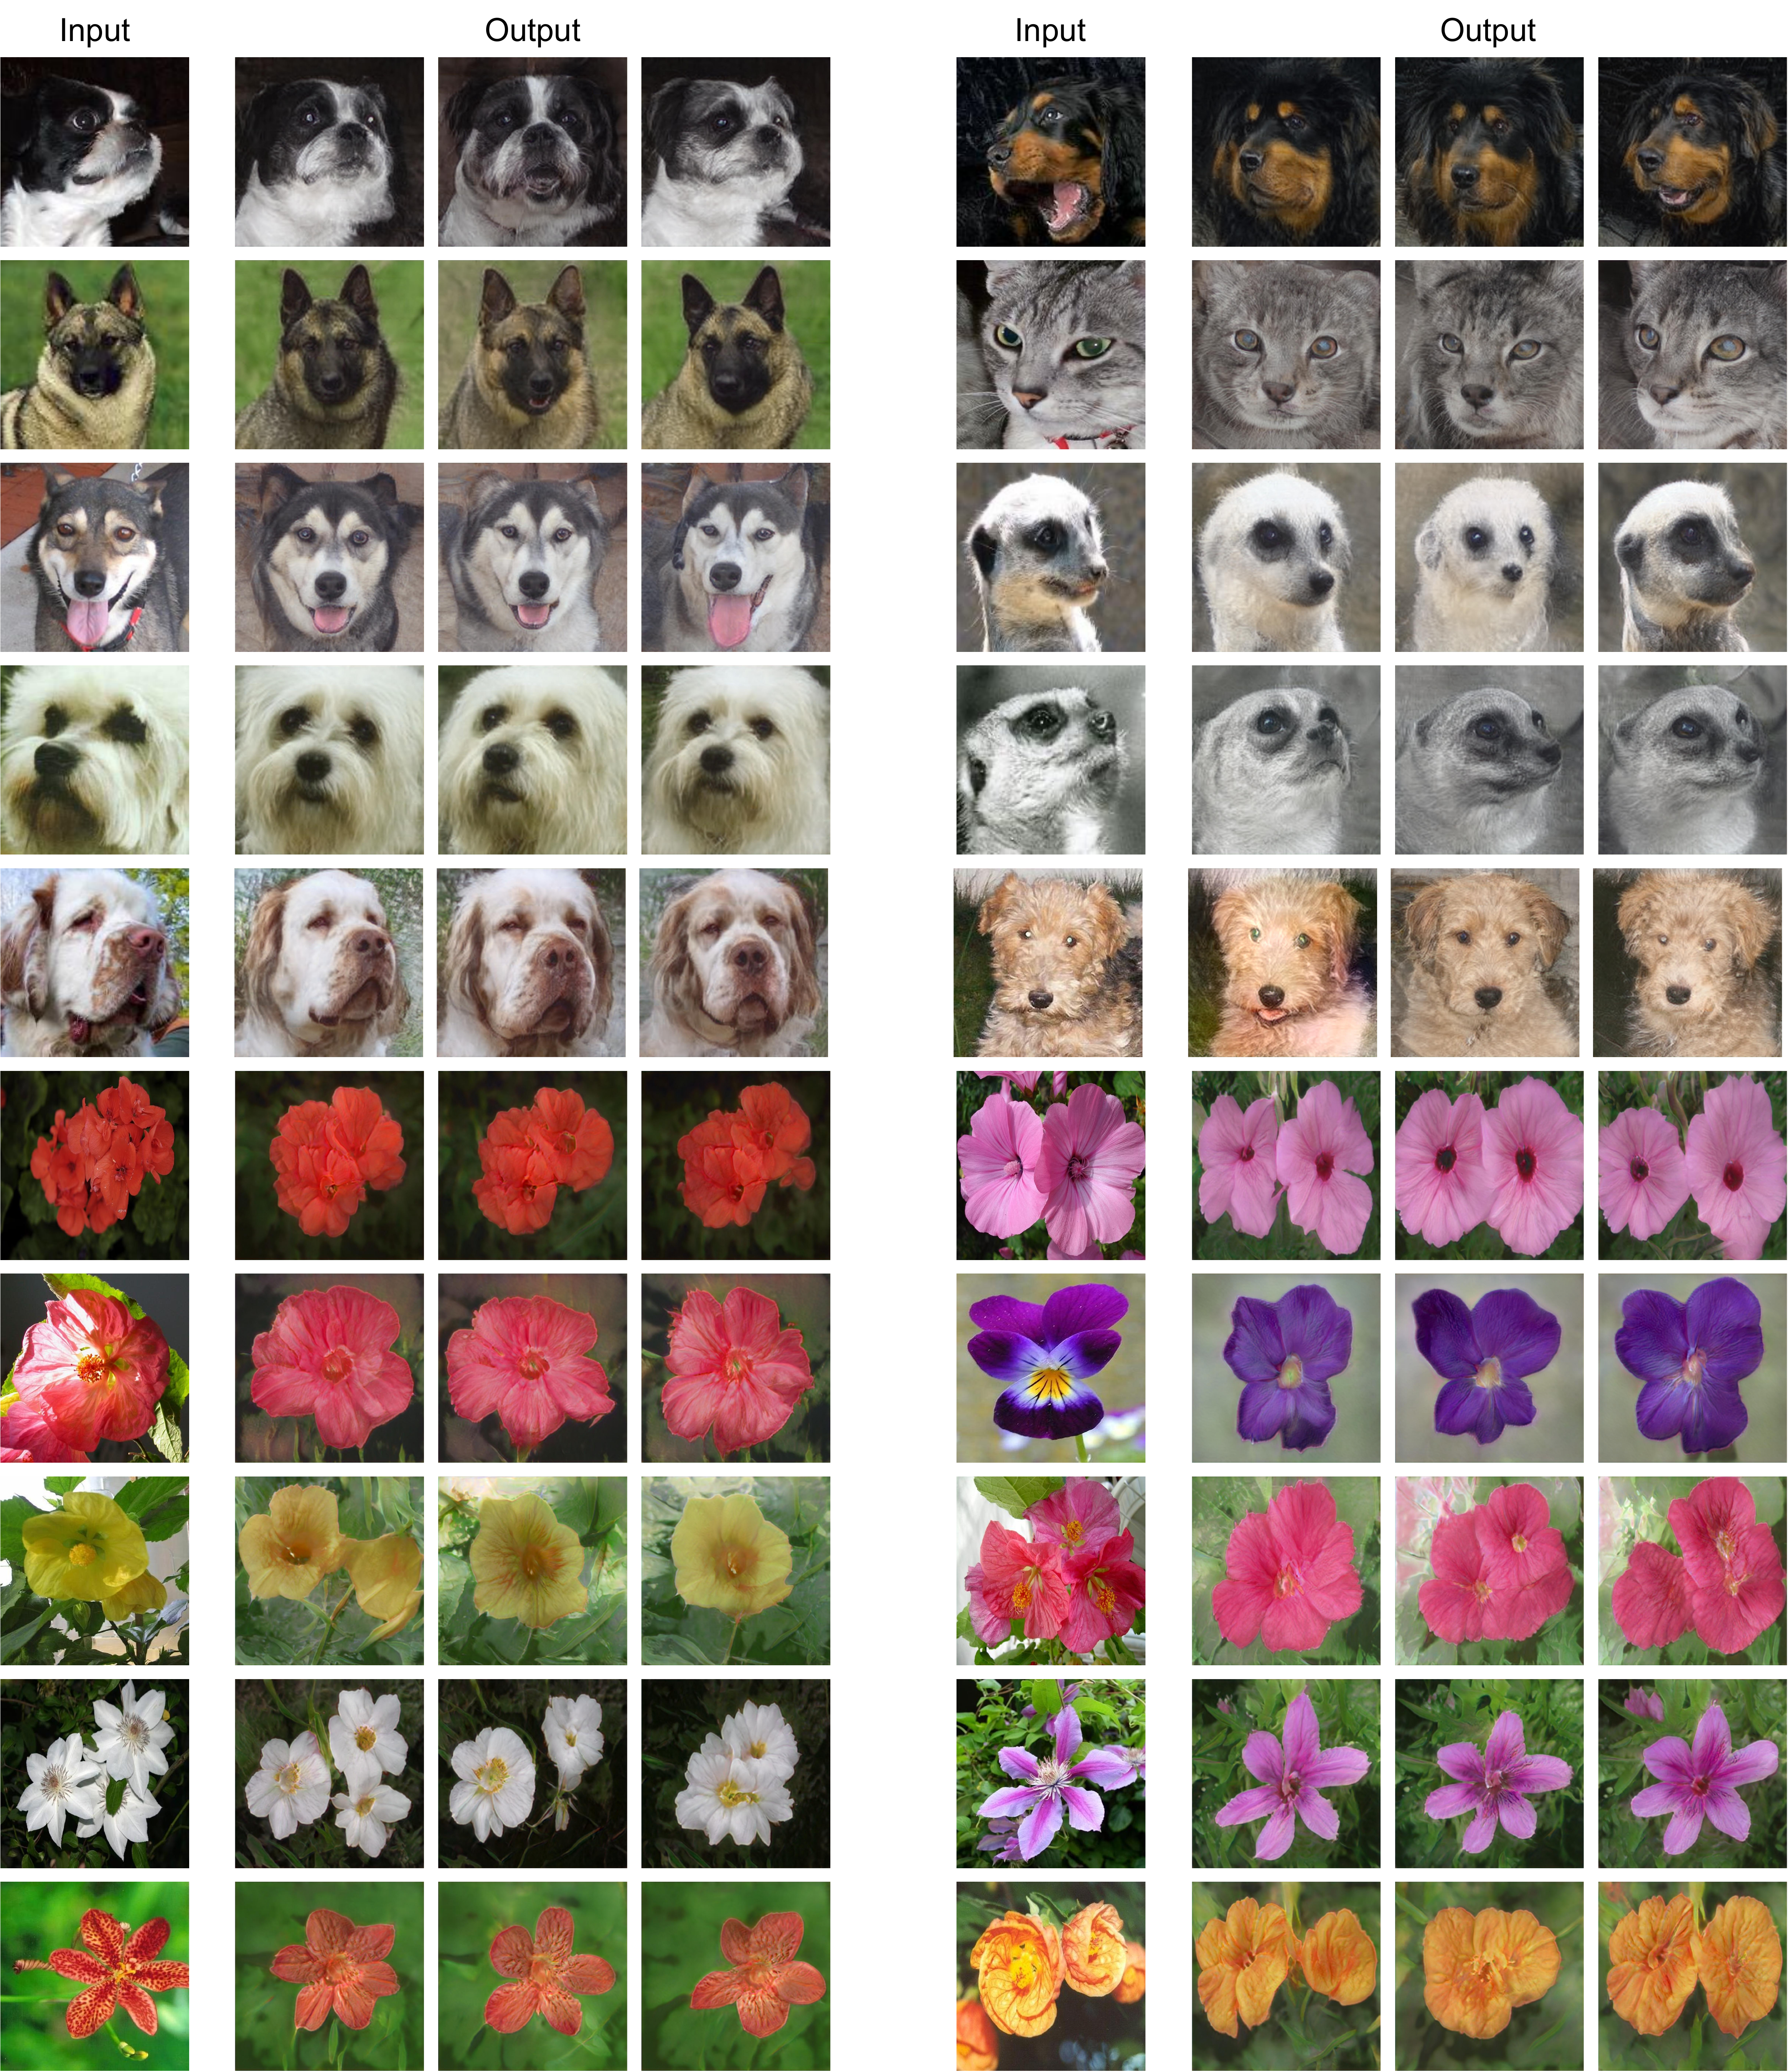}

    \caption{Images generated by SAGE under 1-shot setting on VGGFaces and NABirds.}
    \label{1-shot_samples1}
\end{figure*}

\begin{figure*}[ht]
    \centering
    \includegraphics[width=0.7\linewidth]{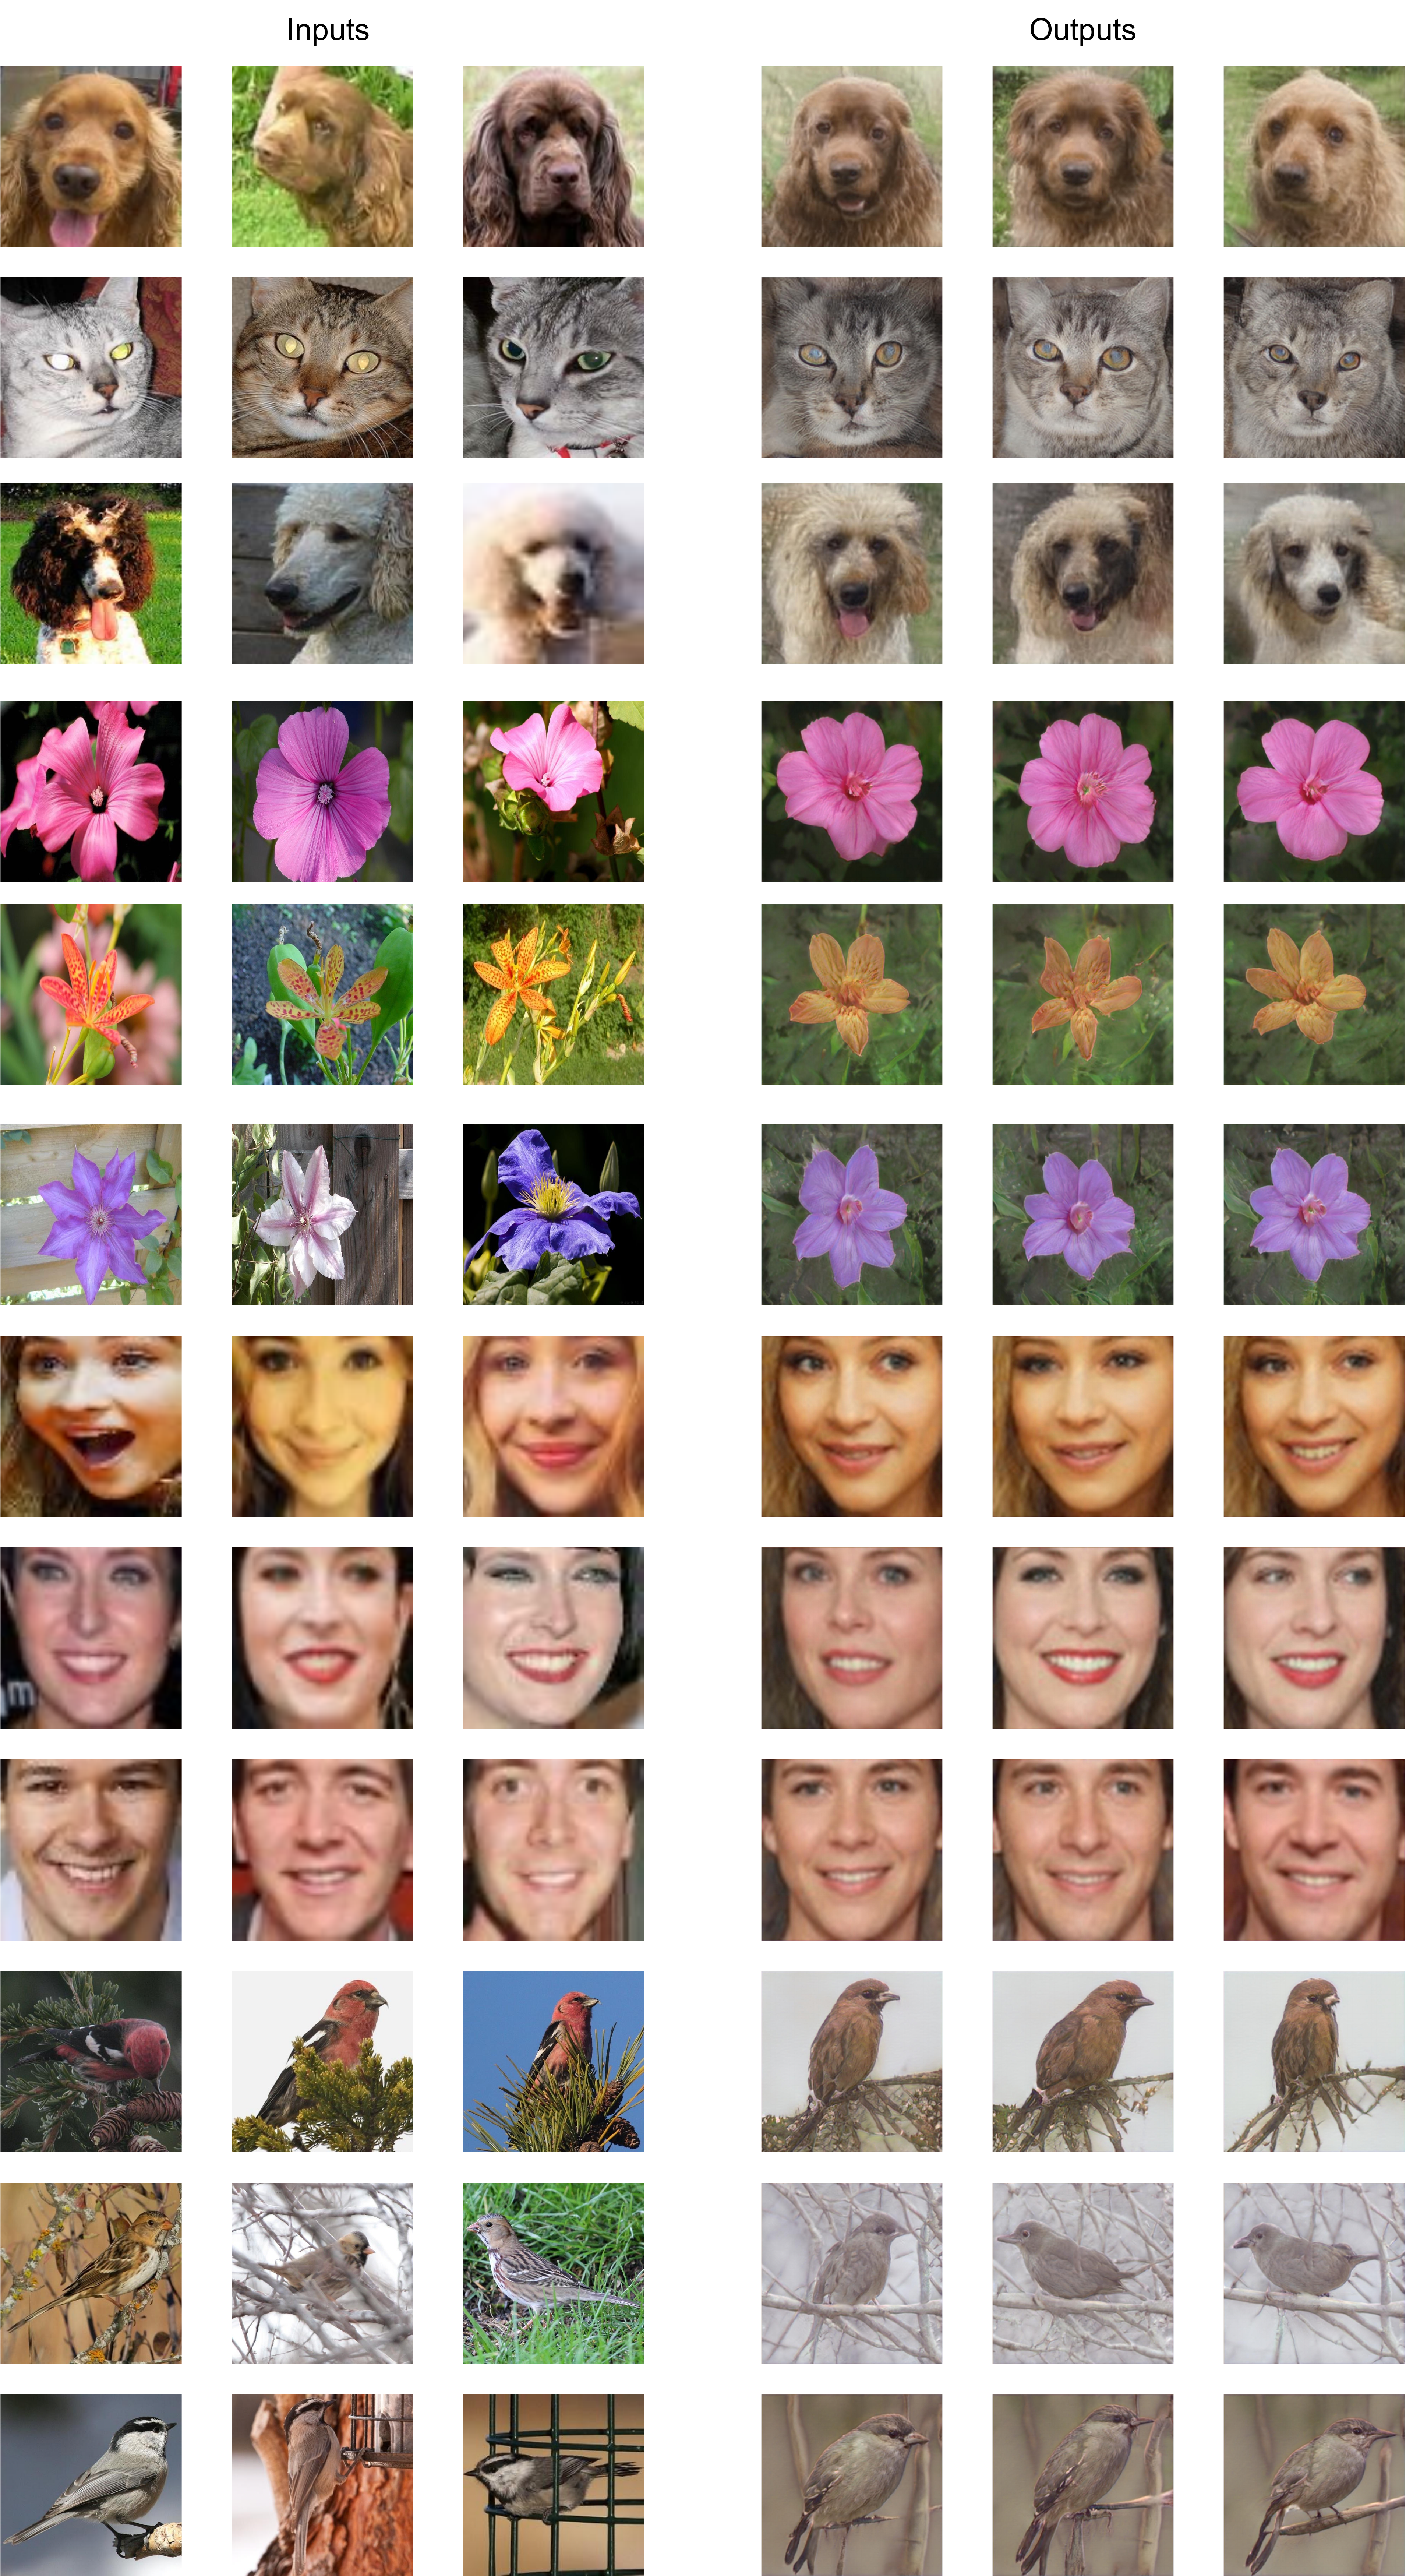}
    \caption{Images generated by SAGE under 3-shot setting on Animal Faces, Flowers, VGGFaces and NABirds.}
    \label{3-shot_samples}
\end{figure*}

\section{Additional Visualizations for SAGE }
\label{good}
We provide more samples generated by SAGE under 1-shot setting in Fig.~\ref{1-shot_samples0} and Fig.~\ref{1-shot_samples1} and under 3-shot setting in Fig.~\ref{3-shot_samples}.
